# Supplementary material for: Towards Efficient Pixel Labeling for Industrial Anomaly Detection and Localization
Source: arXiv:2407.03130 source file (2024-07-04)
Supplement: Supplementary file 1 [file X_suppl.tex]

\clearpage
\setcounter{page}{1}
\maketitlesupplementary

\section{The qualitative comparison on label generation}
\label{sec:label_gen}
In Fig.~\ref{fig:click_mvtec}, we demonstrate the label masks generated by using ADClick model compared with the results obtained by other SOTA Interactive Image Segmentation (IIS) methods including SimplClick \cite{liu_simpleclick_2023} and GPCIS \cite{zhou_interactive_2023}. The experiments are conducted under two training conditions, \emph{i.e.}, the pre-training setting and the fine-tuning setting (shown with $\ast$ symbols); and two click numbers ($3$-click and $5$-click). 
\begin{figure*}[htbp]  
  \centering{
\includegraphics [width=0.99\textwidth]{./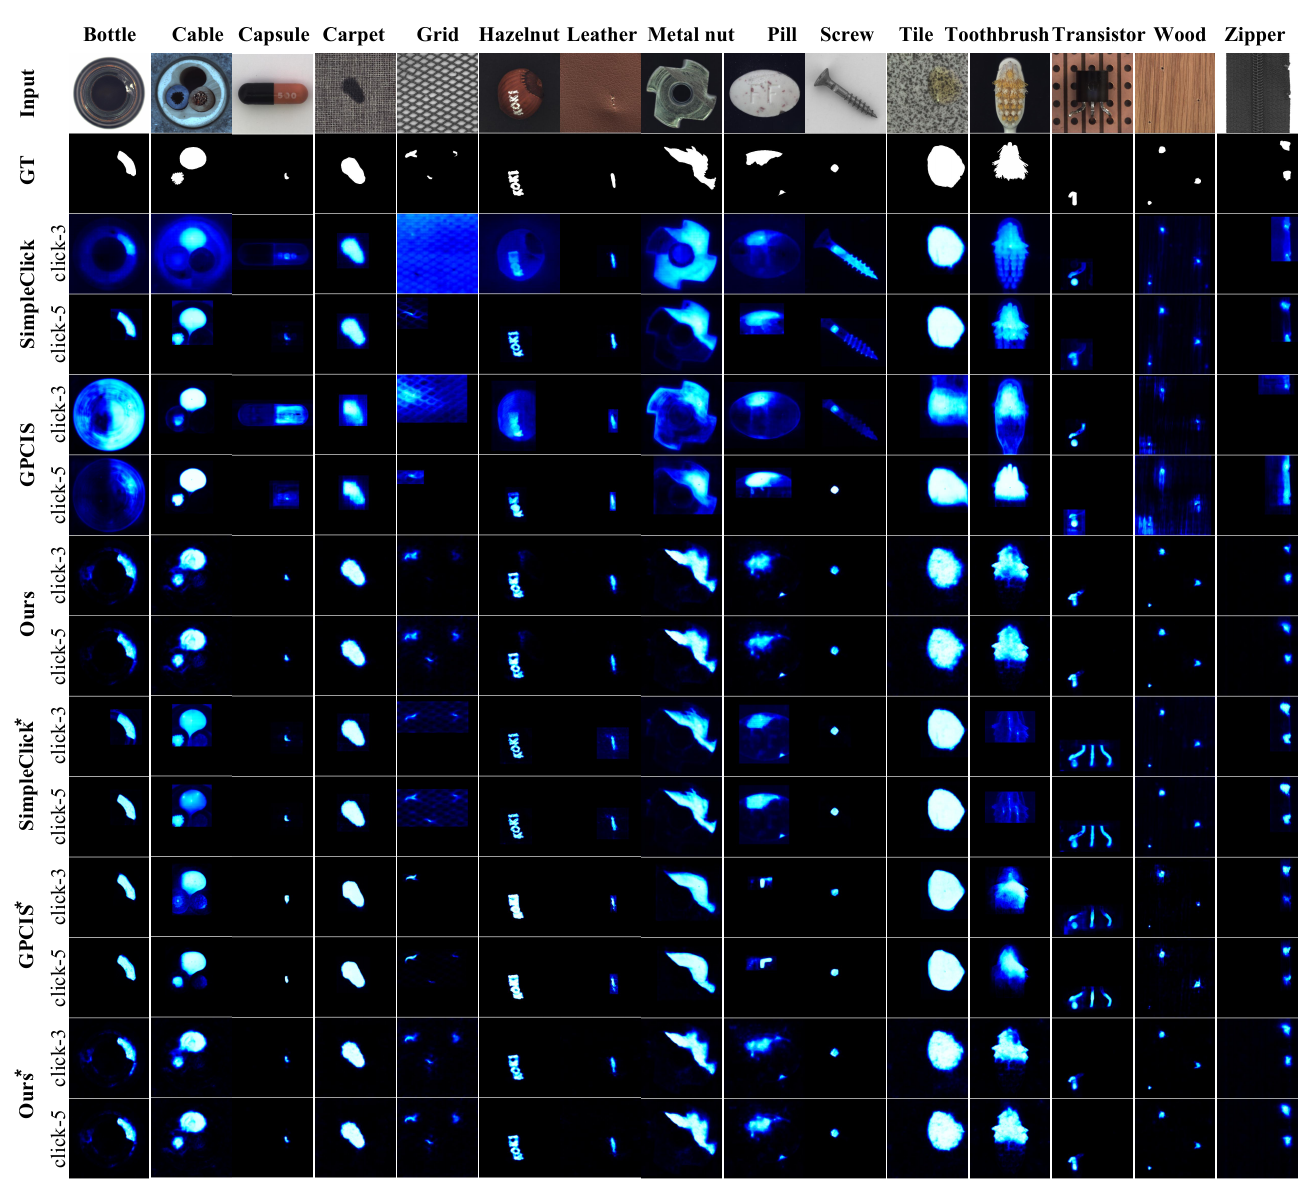}
\caption{The qualitative results of the proposed ADClick algorithm comparing with other IIS methods including SimplClick \cite{liu_simpleclick_2023} and GPCIS \cite{zhou_interactive_2023}.
}
\label{fig:click_mvtec}
}
\end{figure*}

\section{The qualitative comparison on defect detection and localization}
\label{sec:ad}
The anomaly detection and localization results are shown in Fig.~\ref{fig:ad_results}. Four representative AD methods are involved in the comparison, namely the proposed ADClick-Seg, PatchCore \cite{roth2022towards}, DRAEM \cite{zavrtanik2021draem}, and DeSTSeg \cite{zhang2023destseg}, respectively.
\begin{figure*}[htbp]  
  \centering{
\includegraphics [width=0.99\textwidth]{./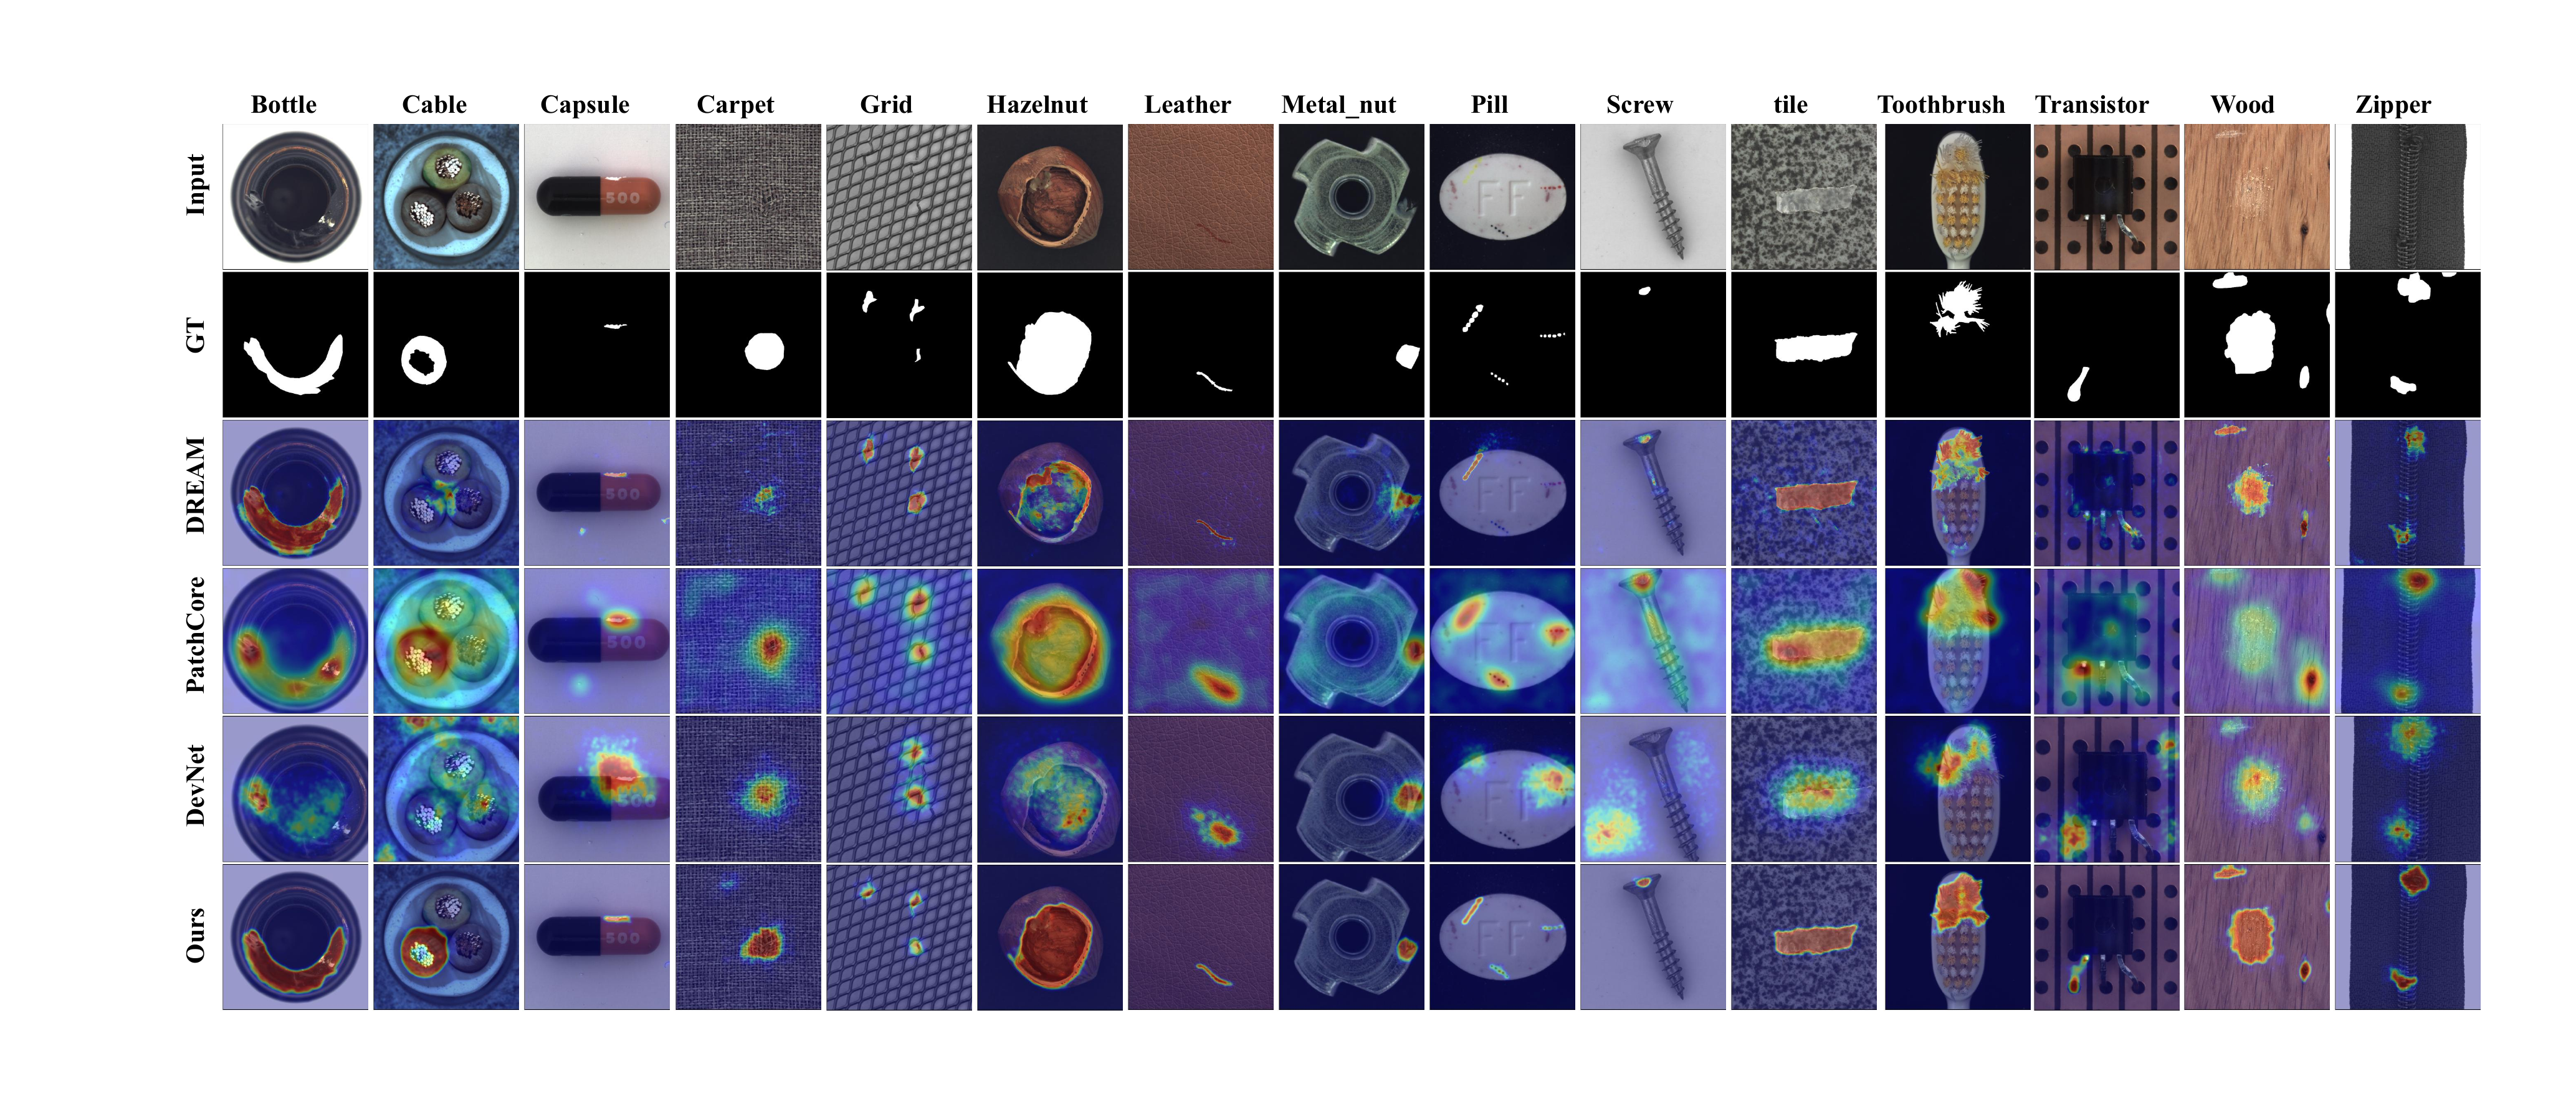}
\caption{The qualitative comparison on anomaly detection and localization of the involved AD methods: the proposed ADClick-Seg, PatchCore \cite{roth2022towards}, DRAEM \cite{zavrtanik2021draem}, and DeSTSeg \cite{zhang2023destseg}.
}
\label{fig:ad_results}
}
\end{figure*}

\section{The proposed labeling tool}
\label{sec:tool}
To further illustrate the validity of the proposed label generation method, we design a ADClick-based labeling tool for anomaly detection and localization. The demonstration video of using the tool is named ``ADClick\_1.mp4'' and supplied as a supplementary file.

\clearpage
% % 
% Having the supplementary compiled together with the main paper means that:
% % 
% \begin{itemize}
% \item The supplementary can back-reference sections of the main paper, for example, we can refer to \cref{sec:intro};
% \item The main paper can forward reference sub-sections within the supplementary explicitly (e.g. referring to a particular experiment); 
% \item When submitted to arXiv, the supplementary will already included at the end of the paper.
% \end{itemize}
% % 
% To split the supplementary pages from the main paper, you can use \href{https://support.apple.com/en-ca/guide/preview/prvw11793/mac#:~:text=Delete%20a%20page%20from%20a,or%20choose%20Edit%20%3E%20Delete).}{Preview (on macOS)}, \href{https://www.adobe.com/acrobat/how-to/delete-pages-from-pdf.html#:~:text=Choose%20%E2%80%9CTools%E2%80%9D%20%3E%20%E2%80%9COrganize,or%20pages%20from%20the%20file.}{Adobe Acrobat} (on all OSs), as well as \href{https://superuser.com/questions/517986/is-it-possible-to-delete-some-pages-of-a-pdf-document}{command line tools}.
